# Supplementary material for: Characterizing the Orientational and Network Dynamics of Polydisperse Nanofibres at the Nanoscale
Source: arXiv:1812.07663 ancillary file (2018-12-18)
Supplement: Supplementary file 1 [file supporting_information.pdf]

# Supporting Information: Characterizing the Orientational and Network Dynamics of Polydisperse Nanofibres at the Nanoscale

Christophe Brouzet,[†,‡] Nitesh Mittal,[†,‡] Fredrik Lundell,[*,†,‡] and L. Daniel Söderberg[†,‡]

†*Linné FLOW Centre, KTH Mechanics, KTH Royal Institute of Technology, Stockholm SE-100 44, Sweden*

‡*Wallenberg Wood Science Center, KTH Royal Institute of Technology, Stockholm SE-100 44, Sweden*

E-mail: frlu@kth.se

## Nanocellulose suspensions

### Preparation

CNC were prepared according to a procedure described recently,[S1] by acid hydrolysis of a never-dried dissolving pulp (from Domsjö AB, Sweden). 20 g of pulp was dispersed in $H_2SO_4$ (175 ml, 64 wt%) and immersed in an oil bath at 45°C for 45 minutes under vigorous magnetic stirring. The reaction mixture was then diluted ten times with deionized water, thoroughly washed through repeated centrifugation and re-dispersion cycles, and dialyzed against deionized water for ten days. Finally, CNC were dispersed by ultrasonication and

filtered on glass filter pore 1 to remove any large aggregates.

For CNF preparation, a well established protocol by Isogai et al.[S2] has been used. In brief, chemically bleached wood fibers (a mixture of 60% Norwegian spruce and 40% Scots pine, provided by Domsjö AB, Sweden) are used. The wood pulp fibers were chemically treated with a 2,2,6,6-tetramethylpiperidinyl-1-oxyl (TEMPO)-mediated oxidation reaction.[S2] CNF dispersions with five different surface charge densities were obtained by varying the conditions on the pulp and/or reaction time followed by homogenization of pulp fibres.[S3,S4] For the preparation of CNF with surface charge densities of 380, 550 and 820 $\mu$mol/g, 1 g of cellulose pulp fibers was suspended in a 0.05 mol/l sodium phosphate buffer (90 ml, pH 6.8), containing TEMPO (16 mg, 0.1 mmol) and sodium chlorite (80%, 1.13 g, 10 mmol). A 2 mol/l sodium hypochlorite solution (0.5 ml) after dilution to 0.1 mol/l with the 0.05 mol/l sodium phosphate buffer was added to the suspension. The suspensions were subsequently stirred at 500 rpm during 1, 2 or 48 hr for surface charge density of 380, 550 or 820 $\mu$mol/g, respectively. For the preparation of the CNF with surface charge densities of 980 and 1360 $\mu$mol/g, wood pulp fibers were suspended at a concentration of 1 wt% in deionized water with the addition of TEMPO (16 mg/g cellulose) and NaBr (100 mg/g cellulose). NaClO (i.e., 2.5 and 5 mmol/g cellulose for surface charge density of 980 and 1360 $\mu$mol/g, respectively) was added dropwise to the suspension under vigorous stirring. The pH of the suspension was maintained at a constant value of 10 by the addition of 0.1 mol/l of NaOH solution until no change in pH value was observed. All the TEMPO-oxidized pulp fibers were washed thoroughly with deionized water by filtration. After the chemical pretreatment, all the TEMPO-oxidized pulp suspensions were passed through a high-pressure homogenizer and CNF suspensions with a concentration higher than 5 g/l were obtained. Finally, these gel-like suspensions were cleaned from the unfibrillated and agglomerated fiber bundles and were diluted by adding deionized water, mixed thoroughly using a mechanical mixer (12000 rpm for 10 min, Ultra Turrax, IKA), and sonicated (10 min, Sonics Vibracell). The diluted suspensions were then centrifuged at 5000 rpm for 60 min followed by the removal of precipitates.

## Characterization in dry state

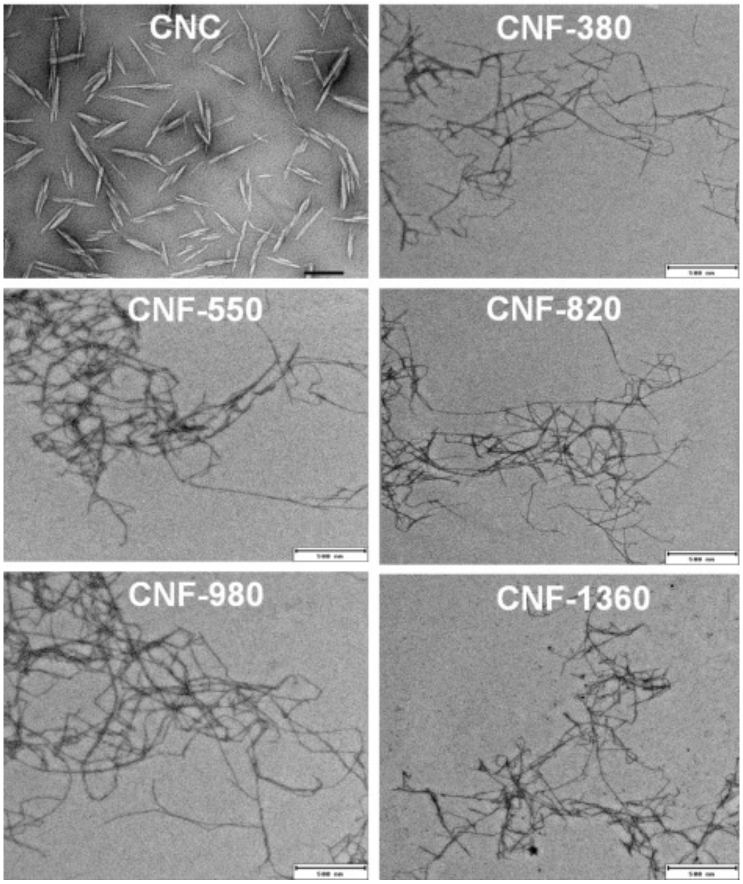


Figure S1: Typical TEM images of CNC and CNF in dry state. Scale bars are 200 nm for CNC and 500 nm for CNF.

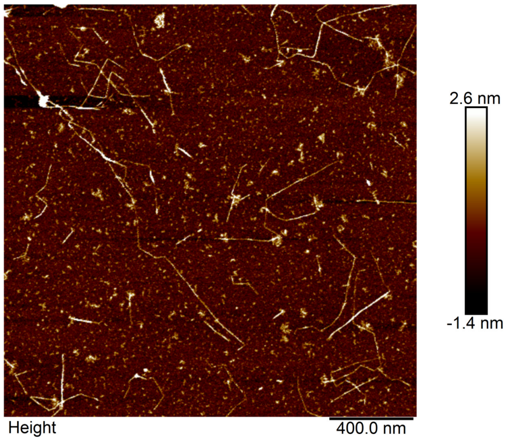


Figure S2: AFM image of nanofibres in dry state.

# Inverse Laplace transform on birefringence decays

As the nanofibre suspensions are polydisperse, nanoparticles of different lengths contribute to the total birefringence. Therefore, after the stop, the birefringence decay can be written as

$$B(t) = \int_0^{+\infty} B^0(L) \exp\left(-6D_r(L)t\right) \mathrm{d}L, \tag{1}$$

where $B^0(L)$ is the contribution of the nanoparticles of length $L$ to the total birefringence signal $B_0 = B(t=0)$ before the flow is stopped. The rotational diffusion coefficient $D_r(L)$ is given by the polydisperse model of Marrucci and Grizzuti[S5,S6] as

$$D_r(L) \approx \frac{\beta k_B T L_*^4}{\eta L^7}, \tag{2}$$

where $\beta$ is a numerical factor, $k_B$ the Boltzmann constant, $T$ the temperature, $L_*$ the entanglement length and $\eta$ the solvent viscosity. The entanglement length $L_*$ is given by

$$L_* = \left(\int_0^{+\infty} \tilde{c}(L) L \ \mathrm{d}L\right)^{-1/2}, \tag{3}$$

with $\tilde{c}$ the concentration distribution.

The birefringence decay described by eq 1 exhibits multiple time scales[S1,S7–S9] as the diffusion coefficient strongly depends on the nanoparticle length $L$. Experimentally, it is therefore plotted with a logarithmic scale in time in order to highlight the different time scales. As eq 1 is a Laplace transform of $B^0(L)$, the contributions of the different lengths to the initial birefringence can be obtained by deconvoluting the decay through an inverse Laplace transform. The method used in this study is inspired from Rogers et al.[S8,S10] and has been described recently.[S1] As it is an ill-posed problem, it requires regularisation procedures. The contributions $B^0(L)$ obtained represent an estimation of the length distribution of the aligned fibrils before the stop. Note that the contribution $B^0(L)$ are not proper distributions, because the area under the curve is equal to the total birefringence before the stop

$B_0 = \int_0^{+\infty} B^0(L)\mathrm{d}L$. Therefore, the comparison with the length distribution obtained from TEM images should be made with respect to shape. To obtain a proper distribution, the contribution $B^0(L)$ has thus to be normalised by $B_0$. The stability of the inverse Laplace transform within the measurement noise can be evaluated by computing error bars on the length distributions, obtained by changing the parameters of the inverse Laplace transform. For all samples, they typically have the size of the symbols used to represent the distributions and are therefore not plotted.

## References


(S1) Brouzet, C.; Mittal, N.; Söderberg, L. D.; Lundell, F. Size-Dependent Orientational Dynamics of Brownian Nanorods. *ACS Macro Lett.* **2018**, *7*, 1022–1027.

(S2) Isogai, A.; Saito, T.; Fukuzumi, H. TEMPO-Oxidized Cellulose Nanofibers. *Nanoscale* **2011**, *3*, 71–85.

(S3) Mittal, N.; Ansari, F.; Gowda V., K.; Brouzet, C.; Chen, P.; Larsson, P. T.; Roth, S. V.; Lundell, F.; Wågberg, L.; Kotov, N. A.; Söderberg, L. D. Multiscale Control of Nanocellulose Assembly: Transferring Remarkable Nanoscale Fibril Mechanics to Macroscale Fibers. *ACS Nano* **2018**, *12*, 6378–6388.

(S4) Geng, L.; Mittal, N.; Zhan, C.; Ansari, F.; Sharma, P. R.; Peng, X.; Hsiao, B. S.; Söderberg, L. D. Understanding the Mechanistic Behavior of Highly Charged Cellulose Nanofibers in Aqueous Systems. *Macromolecules* **2018**, *51*, 1498–1506.

(S5) Marrucci, G.; Grizzuti, N. The Effect of Polydispersity on Rotational Diffusivity and Shear Viscosity of Rodlike Polymers in Concentrated Solutions. *J. Polym. Sci., Polym Lett. Ed.* **1983**, *21*, 83–86.

(S6) Marrucci, G.; Grizzuti, N. Predicted Effect of Polydispersity on Rodlike Polymer

Behaviour in Concentrated Solutions. *J. Non-Newtonian Fluid Mech.* **1984**, *14*, 103–119.

(S7) Chow, A. W.; Fuller, G. G.; Wallace, D. G.; Madri, J. A. Rheooptical Response of Rodlike Chains Subject to Transient Shear Flow. 2. Two-Color Flow Birefringence Measurements on Collagen Protein. *Macromolecules* **1985**, *18*, 793–804.

(S8) Rogers, S. S.; Venema, P.; Sagis, L. M. C.; van der Linden, E.; Donald, A. M. Measuring the Length Distribution of a Fibril System: A Flow Birefringence Technique Applied to Amyloid Fibrils. *Macromolecules* **2005**, *38*, 2948–2958.

(S9) Rosén, T.; Mittal, N.; Roth, S. V.; Zhang, P.; Söderberg, L. D.; Lundell, F. Dynamic Characterization of Dispersed Cellulose Nanofibrils under Process Relevant Conditions. *arXiv.org e-Print archive* **2018**, *1801.07558*, https://arxiv.org/abs/1801.07558.

(S10) Rogers, S. S.; Venema, P.; van der Ploeg, J. P. M.; Sagis, L. M. C.; Donald, A. M.; van der Linden, E. Electric Birefringence Study of an Amyloid Fibril System: The Short End of the Length Distribution. *Eur. Phys. J. E* **2005**, *18*, 207–217.
